# Supplementary material for: BCS Theory in the Weak Magnetic Field Regime for Systems with Nonzero Flux and Exponential Estimates on the Adiabatic Theorem in Extended Quantum Lattice Systems
Source: arXiv:2210.04746 source file (2022-10-10)
Supplement: Supplementary file 1 [file Resolvent_Kernel.tex]

%auto-ignore  % for ArXiv to process correctly

\chapter{The free resolvent kernel}

\begin{refsection}

\section{The fast and rigorous way in \texorpdfstring{$d = 3$}{d=3}}

In $d = 3$, we have that, for $z\in \Cbb$ with $\Re z < 0$ the function $f_z(k) := (z - |k |^2)^{-1}$ is an element of $L^2(\Rbb^3)$ since
\begin{align*}
\int_{\Rbb^3} \bigl| \frac{1}{z - |k|^2}\bigr|^2 \, \dk = 4\pi \int_0^\infty \frac{r^2}{(z + r^2)^2} \, \dr < \infty
\end{align*}
since it is bounded on a finite interval and decays as $r^{-2}$ at infinity. Hence, for $\psi\in L^2(\Rbb^3)$
\begin{align}
\Fcal^{-1} f_z \Fcal \psi = \frac{1}{(2\pi)^{\nicefrac 32}} \cdot \check f_z * \psi \label{Resolvent kernel convolution}
\end{align}
However, $f_z\notin L^1(\Rbb^3)$. Hence, the defining integral can only be understood as an improper Riemann integral in the following way. We have that $f_z \cdot \Idbb_{B_R(0)}\in L^1(\Rbb^3)$ for each $R>0$ and, by dominated convergence, $f_z\Idbb_{B_R(0)}$ converges in $L^2(\Rbb^3)$ to $f_z$. Hence, $\Fcal^{-1}[f_z \cdot \Idbb_{B_R(0)}] \to \check f_z$ in $L^2(\Rbb^3)$. Since $f_z\Idbb_{B_R(0)}\in L^1(\Rbb^3)$, we can compute the inverse Fourier transform directly. As an improper Riemann integral $R\to \infty$, it is given by
\begin{align*}
\check f_z(x) = \frac{1}{(2\pi)^{\nicefrac 32}} \int_{\Rbb^3} \frac{\e^{\i k x}}{z - |k|^2} \, \dd k .
\end{align*}
Employ spherical coordinates, using $x$ as the ``$z$''-direction. We get
\begin{align*}
\check f_z(x) &= \frac{1}{(2\pi)^{\nicefrac 32}}\int_0^\infty \dr \int_0^{2\pi} \dd \varphi \int_0^\pi \dd \theta \; \frac{\e^{\i r|x| \cos(\theta)}}{z - r^2} \cdot r^2\sin(\theta)
\end{align*}
The $\varphi$-integral can be evaluated right away and likewise for the $\theta$-integral. There, we recognize $\sin(\theta)$ to be the inner derivative (apart from factors). Hence
\begin{align*}
\check f_z(x) &= -\frac{1}{\sqrt{2\pi}} \int_0^\infty \dr \; \Bigl[ \frac{\e^{\i r|x|\cos(\theta)}}{\i r |x|(z - r^2)} \cdot r^2\Bigr]_{\theta = 0}^{\theta =\pi} \\
&= - \frac{1}{\sqrt{2\pi} \cdot \i |x|} \int_0^\infty \dr \; \frac{r}{z - r^2} \bigl[ \e^{-\i r |x|} - \e^{\i r |x|}\bigr]
\end{align*}
In the first integral, we perform a change of variables $r \mapsto -r$ so that
\begin{align*}
\int_0^\infty \dd r \;\frac{r}{z - r^2} \cdot \e^{-\i r|x|} = \int_0^{-\infty} \dr \; \frac{r}{z - r^2}\cdot \e^{\i r|x|} = -\int_{-\infty}^0 \dr \; \frac{r}{z - r^2}\cdot \e^{\i r|x|}.
\end{align*}
Hence, we get
\begin{align*}
\check f_z(x) &= \frac{1}{\sqrt{2\pi} \cdot \i |x|} \cdot \int_{-\infty}^\infty \dr \; \frac{r \cdot \e^{\i r|x|}}{z - r^2}.
\end{align*}
This integral we solve by using the residue theorem on the function $f(w) := \frac{w\cdot \e^{\i w|x|}}{z + w^2}$.  Let $R>0$ such that the roots of the denominator $w = \pm \i \sqrt{-z}$ lie inside $B_R(0)$. Then choose the contour $\gamma_R := \gamma_1 \dot + \gamma_2$ with $\gamma_1(t) = t$, $t\in [-R,R]$ and $\gamma_2(t) = R\e^{\i t}$, $t\in [0,\pi]$. Consider the contribution of the arch $\gamma_2$
\begin{align*}
\int_0^\pi \Bigl| \frac{R\cdot \e^{\i t}\cdot \e^{\i R\e^{\i t} |x|}}{z - (R\e^{\i t})^2}\Bigr| \, \dt\leq \int_0^\pi \frac{R\cdot \e^{-R\sin(t)|x|}}{R^2 - z} \, \dt \xra{R\to\infty} 0
\end{align*}
Hence, we have that
\begin{align*}
\int_{-\infty}^\infty \frac{r \cdot \e^{\i r |x|}}{z - r^2} \, \dr = \frac{2\pi\i \cdot \i \sqrt{-z}\cdot \e^{\i \cdot \i \sqrt{-z} \cdot |x|}}{-2 \i \sqrt{-z}} = - \pi \i  \cdot \e^{-\sqrt{-z}\cdot |x|}
\end{align*}
We obtain the final result
\begin{align*}
\check f_z(x) = -\frac{1}{\sqrt{2\pi} \cdot \i |x|} \cdot  \pi \i \cdot \e^{-\sqrt{-z}\cdot |x|} = -\sqrt{\frac{\pi}{2}} \cdot \frac{\e^{-\sqrt{-z}\cdot |x|}}{|x|}
\end{align*}
Defining
\begin{align}
G^z(x) := \frac{1}{(2\pi)^{\nicefrac 32}} \cdot \check f_z(x) = -\frac{1}{4\pi \cdot |x|}\cdot \e^{-\sqrt{-z}\cdot |x|} \label{Resolvent kernel 3d}
\end{align}
we finally get from \eqref{Resolvent kernel convolution} that
\begin{align*}
(z + \Delta)^{-1} \psi = G^z * \psi 
\end{align*}

\section{Via Bessel functions}

In this section, we want to compute the resolvent kernel of the free Laplacian $-\Delta -\mu$ for $\mu\in \Rbb$ in $L^2(\Rbb^3)$. Parts of this can be found in \cite[p. 202]{Teschl}. For a moment, we are working with arbitrary dimension $d\geq 1$ but for concrete computations, we will soon put $d =3$. Our aim is to show that the kernel of $(z + \Delta)^{-1}$ is given by the function $K(x-y) = G^z(|x-y|)$, where
\begin{align*}
G^z(r) := -\frac{1}{4\pi r} \cdot \e^{-\sqrt{-z}\cdot (r-\mu)} \qquad \qquad z\in \Cbb \setminus [0,\infty) , \quad r\geq 0.
\end{align*}

\subsubsection{The heat semigroup}

The first step is to calculate the heat semigroup $\e^{-t H_0}$ of the Laplacian $H_0 := -\Delta$ for all $t\geq 0$. Let $\psi\in L^2(\Rbb^d)$, let $t\geq 0$ and $\varepsilon>0$. To generate decay also for $t =0$, for $k\in \Rbb^d$, introduce an approximation
\begin{align*}
j_\varepsilon(|k|^2) := \e^{-(t + \varepsilon)|k|^2}.
\end{align*}
Then $j_\varepsilon$ is uniformly bounded in $\varepsilon>0$ and $j_\varepsilon(|k|^2) \to \e^{-t |k|^2}$ as $\varepsilon\to 0$ pointwise\footnote{This computation will eventually become nonrigorous and we will only verify in the end that the obtained operator will indeed be the resolvent. However, to be a little bit more convincing, let us be precise at least in this first part.}. Hence, by the functional calculus, we get that $j_\varepsilon(H_0)\psi \to \e^{-t H_0}\psi$ strongly. Since $j_\varepsilon(|\cdot|^2)$ belongs to $\Scal(\Rbb^d)$, we may apply the convolution theorem to obtain
\begin{align*}
j_\varepsilon(H_0)\psi = \Fcal^{-1} j_\varepsilon(|\cdot|^2) \Fcal\psi = \check{j_\varepsilon \cdot \hat \psi} = \frac 1{(2\pi)^{\nicefrac d2}} \cdot \check j_\varepsilon * \psi
\end{align*}
Hence, we need to compute $L^2$-limits of the object $\check j_\varepsilon$. 
%Now, Young's convolution inequality says that if $f\in L^p(\Rbb^d)$ and $g\in L^q(\Rbb^d)$, then $f* g\in L^r(\Rbb^d)$ with $\frac{1}{p} + \frac 1q = \frac 1r+ 1$ and
%\begin{align*}
%\Vert f* g\Vert_{L^r(\Rbb^d)} \leq \Vert f\Vert_{L^p(\Rbb^d)} \cdot \Vert g\Vert_{L^q(\Rbb^d)}
%\end{align*}
The first step is to compute the Fourier inverse transform of $k \mapsto j_\varepsilon(|k|^2)$. Since this function is Schwartz, we have
\begin{align*}
\check j_\varepsilon(x) = \frac{1}{(2\pi)^{\nicefrac d2}} \int_{\Rbb^d} \dk \; \e^{\i k x} \e^{-(t + \varepsilon) |k|^2}
\end{align*} 
The quadratic expansion reads\footnote{Note that this is the Euclidean (i.e., $\Rbb$-linear) scalar product and not the $\Cbb$-linear one.}
\begin{align*}
-(t + \varepsilon) \Bigl| k - \frac{\i x}{2(t + \varepsilon)} \Bigr|^2 &= -(t + \varepsilon) \Bigl[|k|^2 - \frac{\i kx}{t + \varepsilon} - \frac{|x|^2}{4(t+\varepsilon)^2}\Bigr] \\
&= -(t + \varepsilon)|k|^2 + \i kx + \frac{|x|^2}{4(t +\varepsilon)}
\end{align*}
and yields
\begin{align}
\check j_\varepsilon(x) = \frac{1}{(2\pi)^{\nicefrac d2}} \cdot \e^{-\frac{|x|^2}{4(t+\varepsilon)}} \cdot \int_{\Rbb^d} \dd k\; \e^{- (t+\varepsilon) |k - \frac{\i x}{2(t+\varepsilon)}|^2} \label{jeps-convolution}
\end{align}
Now, we claim that
\begin{align}
\check j_\varepsilon(x) = \frac{1}{(2\pi)^{\nicefrac d2}} \cdot \e^{-\frac{|x|^2}{4(t+\varepsilon)}} \cdot \int_{\Rbb^d} \dd k \; \e^{-(t + \varepsilon)|k|^2} \label{jeps mit Cauchy}
\end{align}
To verify this, we make use of Cauchy's integral theorem. It suffices to consider the one-dimensional case due to the factorization of the integrand. Hence, our object of interest is
\begin{align*}
\int_{-\infty}^\infty \dd k \; \e^{-(t + \varepsilon)k^2} = \lim_{R\to\infty} \int_{-R}^R \e^{-(t + \varepsilon)k^2} = \lim_{R\to\infty} \int_{\gamma_R} \dd w \; f(w)
\end{align*}
with the analytic function $f(w) := \e^{-(t + \varepsilon)w^2}$ and the path $\gamma_R(t) := s$ for $s\in [-R,R]$. Define the path $\tilde \gamma_R(t) := s - \frac{\i x}{2(t + \varepsilon)}$ as well as the joining paths $\gamma_1,\gamma_2\colon [0,1] \lra \Cbb$ with
\begin{align*}
\gamma_1(s) &:= -R - \frac{\i xs}{2(t + \varepsilon)} & \gamma_2(s) &:= R - \frac{\i x(1-s)}{2(t + \varepsilon)}
\end{align*}
Since $f$ is analytic, Cauchy's integral theorem says that for $\Gamma_R := \gamma_1 \mathop{\dot +} \tilde \gamma_R  \mathop{\dot +} \gamma_2 \mathop{\dot -} \gamma_R$, we obtain
\begin{align*}
0 = \int_{\Gamma_R} \dd w \; f(w) = \int_{\tilde \gamma_R} \dd w\; f(w) - \int_{\gamma_R}\dd w\; f(w) + \int_{\gamma_1 \dot + \gamma_2} \dd w\; f(w)
\end{align*}
Thus, our task is to show that the parts of $\gamma_1$ and $\gamma_2$ vanish in the limit $R\to\infty$. For $\gamma_1$, we have
\begin{align*}
\Bigl|\int_{\gamma_1} \dd w \; f(w) \Bigr| &\leq \int_0^1 \ds \; \bigl|\e^{-(t+ \varepsilon) (-R - \frac{\i xs}{2(t+\varepsilon)})^2}\bigr| = \int_0^1 \ds \; \e^{-(t + \varepsilon)(R^2 + \frac{x^2s^2}{4(t + \varepsilon)^2})} \leq \e^{-\varepsilon R^2}
\end{align*}
and concerning $\gamma_2$, we obtain
\begin{align*}
\Bigl|\int_{\gamma_2} \dd w \; f(w) \Bigr| &\leq \int_0^1 \ds \; \bigl|\e^{-(t+ \varepsilon) (R - \frac{\i x(1-s)}{2(t+\varepsilon)})^2}\bigr| = \int_0^1 \ds \; \e^{-(t + \varepsilon)(R^2 + \frac{x^2(1-s)^2}{4(t + \varepsilon)^2})} \leq \e^{-\varepsilon R^2}
\end{align*}
Hence, taking the limit $R\to\infty$, we get that
\begin{align*}
\int_\Rbb \dd k \; \e^{-(t + \varepsilon)k^2 } = \int_\Rbb \dd k \; \e^{-(t + \varepsilon) |k - \frac{\i x}{2(t + \varepsilon)}|^2}.
\end{align*}
Using \eqref{jeps mit Cauchy} and computing the remaining integral, we finally get
\begin{align*}
\check j_\varepsilon(x) = \frac{1}{(2\pi)^{\nicefrac d2}}\cdot  \e^{-\frac{|x|^2}{4(t + \varepsilon)}} \cdot \Bigl( \frac{\pi}{t+\varepsilon}\Bigr)^{\nicefrac d2} = \frac{1}{(2(t+\varepsilon))^{\nicefrac d2}} \cdot  \e^{-\frac{|x|^2}{4(t+\varepsilon)}}
\end{align*}
or, put differently
\begin{align*}
j_\varepsilon(H_0) \psi(x) = \frac{1}{(4\pi(t +\varepsilon))^{\nicefrac d2}} \int_{\Rbb^d} \e^{-\frac{|x-y|^2}{4(t+\varepsilon)}} \cdot \psi(y)\, \dy
\end{align*}

\subsubsection{A resolvent identity}

For $z\in \Cbb$ with $\Re z < 0$, consider the identity
\begin{align*}
\int_0^r \e^{zt} \e^{-t H_0} \dt = (z - H_0)^{-1} \bigl[ \e^{zr} \e^{-r H_0} - \Idbb\bigr] \xra{r\to\infty} - (z - H_0)^{-1}
\end{align*}
in operator norm. This follows from the functional calculus. It follows from Fubini that
\begin{align*}
\e^{-\varepsilon H_0} (z - H_0)^{-1} \psi(x) &= -\int_0^\infty \e^{zt}\e^{-(t+\varepsilon)H_0} \psi(x) \, \dt \\
&= - \int_0^\infty \dt \; \frac{1}{(4\pi(t + \varepsilon))^{\nicefrac d2}} \int_{\Rbb^d} \dy \; \e^{zt}  \e^{-\frac{|x-y|^2}{4(t+\varepsilon)}} \cdot \psi(y)\\
&= \int_{\Rbb^d} \dy\; \Bigl( \int_0^\infty \dt\; \frac{1}{(4\pi(t + \varepsilon))^{\nicefrac d2}} \cdot \e^{zt}  \e^{-\frac{|x -y|^2}{4(t+\varepsilon)}}\Bigr)\cdot \psi(y)
\end{align*}
Hence, the operator $\e^{-\varepsilon H_0}(z - H_0)^{-1}$ has the kernel $K_\varepsilon(|x-y|)$ with
\begin{align*}
K_\varepsilon(r) := \int_0^\infty \dt \; \frac{1}{(4\pi(t + \varepsilon))^{\nicefrac d2}} \cdot \e^{zt} \e^{-\frac{r^2}{4(t+\varepsilon)}}   = \e^{-z\varepsilon} \int_\varepsilon^\infty \dt\; \frac{1}{(4\pi t)^{\nicefrac d2}} \cdot \e^{zt} \e^{-\frac{r^2}{4t}}, \qquad  r\in \Rbb.
\end{align*}
Note that, formally, we can take the limit as $\varepsilon \to 0$ for each $r > 0$. We do this now, disrespecting the convergence we would need so that \eqref{jeps-convolution} would really converge to the desired object. We will confirm in the end that our so-obtained operator is indeed the resolvent. Taking the limit $\varepsilon \to 0$ for $r>0$ gives the resolvent kernel of the free Laplacian
\begin{align*}
G^z(r) = \int_0^\infty \dt \; \frac{1}{(4\pi t)^{\nicefrac d2}} \cdot \e^{zt}\e^{-\frac{r^2}{4t}} \qquad \qquad r>0, \; \Re z < 0.
\end{align*}
Now, let us assume that $z\in \Rbb$, $z < 0$ for the moment. We will later show that the formulas hold for the remaining $\Re z < 0$ by the identity theorem. Note that $\sqrt{-z}$ is a well-defined real number. Perform a change of variables $s := \log (\frac{2t\sqrt{-z}}{r})$ so that $t = \e^s \frac{r}{2\sqrt{-z}}$. Hence, $\dt = \e^s \frac{r}{2\sqrt{-z}} \dd s$ and we obtain
\begin{align*}
G^z(r) &= -\frac{1}{(4\pi)^{\nicefrac d2}} \int_{-\infty}^\infty \ds \; \Bigl( \e^{-s} \frac{2\sqrt{-z}}{r}\Bigr)^{\nicefrac d2} \e^{-\frac{r^2 \cdot 2\sqrt{-z}}{4 \e^s\cdot r} + \frac{z\e^s\cdot r}{2\sqrt{-z}} } \cdot \e^s \frac{r}{2\sqrt{-z}} \\
&= - \frac{1}{(4\pi)^{\nicefrac d2}} \Bigl( \frac{2\sqrt{-z}}{r}\Bigr)^{\nicefrac d2-1} \int_{-\infty}^\infty \e^{-s(\nicefrac d2 - 1)} \e^{-r\sqrt{-z} \cosh(s)} \, \ds
\end{align*}
Hence, defining the spherical Bessel function for $\nu\in \Rbb$ and $x >0$ as
\begin{align*}
K_\nu(x) := \frac 12 \int_{-\infty}^\infty \e^{s\nu} \e^{-x\cosh(s)} \, \ds
\end{align*}
we get that
\begin{align}
G^z(r) = - \frac{1}{2\pi} \Bigl( \frac{\sqrt{-z}}{2\pi r}\Bigr)^{\nicefrac d2 -1} K_{\frac d2-1}\lk r\sqrt{-z}\rk \label{Resolvent with Bessel}
\end{align}
We are going to show in the next section \ref{Bessel functions} that $d = 3$ gives
\begin{align*}
K_{\frac 12}(x) = K_{\frac 32 - 1}(x) = \sqrt{\frac{\pi}{2x}} \cdot \e^{-x},
\end{align*}
see \eqref{Konehalf final representation}, so that, applying \eqref{Resolvent with Bessel}, we finally obtain the result\footnote{Note that the sign comes from our different sign convention in $(z - H_0)^{-1}$ as opposed to the standard literature. There, we have $(H_0 - z)^{-1}$ and no sign correspondingly in $G^z(r)$.}
\begin{align*}
G^z(r) = - \frac{1}{2\pi} \sqrt{\frac{\sqrt{-z}}{2\pi r} } \cdot \sqrt{\frac{\pi}{2 r\sqrt{-z} }} \cdot \e^{-r \sqrt{-z}} = - \frac{1}{4\pi r} \e^{-\sqrt{-z} \cdot r}
\end{align*}

\subsection{Bessel functions}
\label{Bessel functions}

In this section, we want to compute $K_\nu$ for $\nu = \frac d2 -1$. Of course, we are essentially interested in $d = 3$ but we keep the discussion as general as possible. All we do is from \cite{Schnizer}.

The $\mu$\tho -order Bessel differential equation reads
\begin{align}
\frac{\dd^2 Z_\mu(x)}{\dd x^2} + \frac{1}{x} \cdot \frac{\dd Z_\mu(x)}{\dd x} + \Bigl( 1- \frac{\mu^2}{x^2} \Bigr) Z_\mu(x) = 0 \label{Bessel equation}
\end{align}
We have the following set of solutions to \eqref{Bessel equation}
\begin{align*}
J_\mu(x) := \Bigl( \frac{x}{2}\Bigr)^\mu \sum_{k=0}^\infty \frac{(-1)^k}{k!\cdot \Gamma(\mu + k +1)} \Bigl( \frac{x}{2}\Bigr)^{2k}
\end{align*}
Here, $J_\mu$ and $J_{-\mu}$ are linear independent if and only if $\mu$ is not an integer. Hence, for odd dimensions $d$, since $\mu = \nicefrac d2 -1$, this is the case. For simplicity we will stick to this case. Also introduce the modified Bessel differential equation of $\mu$\tho -order:
\begin{align}
\frac{\dd^2 Z_\mu(x)}{\dd x^2} + \frac{1}{x} \cdot \frac{\dd Z_\mu(x)}{\dd x} - \Bigl( 1+ \frac{\mu^2}{x^2} \Bigr) Z_\mu(x) = 0 \label{Bessel modified equation}
\end{align}
Define the functions
\begin{align}
H_\mu^{(1)} := \frac{J_{-\mu} - \e^{\mp \i \mu \pi} J_\mu}{\i \sin (\mu \pi)} \label{Hmu definition}
\end{align}
Then, the claim is that the functions
\begin{align}
K_\mu(x) := \frac{\pi\i}{2} \e^{\frac{\i\pi \mu}{2}} H_\mu^{(1)}(\e^{\frac{\i \pi}{2}} x) \label{Kmu definition}
\end{align}
solve \eqref{Bessel modified equation}. There is also an integral representation 
\begin{align}
K_\mu(x) = \frac 12 \int_{-\infty}^\infty \ds \; \e^{-\mu s} \e^{-x\cosh(s)} \label{Kmu integral rep}
\end{align}

We are going to compute $K_\mu$ using the representation \eqref{Kmu definition}. To verify that this is equal to the integral representation \eqref{Kmu integral rep} we show that both representations satisfy the differential equation \eqref{Bessel modified equation}, which is locally Lipschitz continuous. Hence, the two functions must coincide. As a preparation, however, we need to collect a fact about the Gamma function $\Gamma$. Also, we rather prove that $J_\mu$ satisfies \eqref{Bessel equation}. As a Corollary, the assertion about $K_\mu$ will follow.

\subsubsection{Functional equation for the Gamma function}

Recall that the $\Gamma$-function is defined by
\begin{align}
\Gamma(z) := \int_0^\infty t^{z - 1} \e^{-t} \, \dt \label{Gamma-function}
\end{align}
It is a one liner to prove that for $k\in \Rbb$, $k\geq -\mu$,
\begin{align}
\Gamma((k-1) + \mu + 1) = \frac{\Gamma(k+\mu + 1)}{k + \mu}. \label{functional equation Gamma}
\end{align}
This follows from
\begin{align*}
\Gamma(k + \mu + 1) &= \int_0^1 t^{k + \mu + 1 - 1} \e^{-t} \, \dt = -t^{k+\mu + 1 - 1} \e^{-t} \Big|_0^\infty + \int_0^\infty t^{k + \mu -1}(k + \mu) \e^{-t} \, \dt \\
&= (k + \mu) \Gamma(k + \mu).
\end{align*}

\subsubsection{The functions \texorpdfstring{$J_\mu$}{Jmu} are solutions to \texorpdfstring{(\ref{Bessel equation})}{(\ref{Bessel equation})}}

Note that by performing an index shift $k \to k -1$ and using the above relation about $\Gamma$, we have the alternative representation
\begin{align*}
J_\mu(x) = \sum_{k=0}^\infty \frac{(-1)^k}{k! \cdot \Gamma(k + \mu + 1)} \Bigl( \frac x2\Bigr)^{2k + \mu} = \sum_{k=1}^\infty \frac{(-1)^{k-1} k(k+\mu)}{k! \cdot  \Gamma(k + \mu + 1)} \Bigl( \frac x2\Bigr)^{2k+\mu -2}
\end{align*}
We need this later to insert into the differential equation. Since $J_\mu$ is an entire function, compute the first derivative termwise to get
\begin{align*}
J_\mu'(x) = \sum_{k=0}^\infty \frac{(-1)^k (2k+\mu) x^{2k+ \mu -1}}{k! \cdot  J(k + \mu + 1) \cdot 2^{2k+\mu}}
\end{align*}
and likewise we compute the second derivative
\begin{align*}
J_\mu''(x) &= \sum_{k=0}^\infty \frac{(-1)^k (2k+\mu) (2k+\mu - 1)\cdot  x^{2k+\mu -2}}{k! \cdot \Gamma(k +\mu + 1) \cdot 2^{2k+\mu}}
\end{align*}
Inserting these computations into \eqref{Bessel equation}, we obtain
\begin{align*}
x^2 J_\mu''(x) + x J_\mu'(x) + (x^2 - \mu^2) J_\mu(x) = \hspace{-150pt}& \\
&= \sum_{k=0}^\infty \frac{(-1)^k}{k! \cdot \Gamma(k + \mu - 1)} \frac{x^{2k+\mu}}{2^{2k+\mu}} \bigl[ (2k + \mu)(2k + \mu - 1) + 2k + \mu - 4k(k + \mu) - \mu^2\bigr]
\end{align*}
Considering the term in square brackets, we see that
\begin{align*}
(2k + \mu)^2 - 4k(k + \mu) - \mu^2 &= 4k^2 + 4\mu k + \mu^2 - 4k^2 - 4\mu k - \mu^2 =0
\end{align*}
Hence, we indeed do have a solution.

\subsubsection{\texorpdfstring{$K_\mu$}{Kmu} are solutions in both representations}

To see that $K_\mu$ as in \eqref{Kmu definition} is a solution of \eqref{Bessel modified equation}, we just need to prove that the function $\tilde J_\mu (x) := J_\mu(\i x)$ solves \eqref{Bessel modified equation}. The rest is linearity of \eqref{Bessel modified equation}. Since $\tilde J_\mu'(x) = \i J_\mu'(\i x)$ and $\tilde J_\mu''(x) = - J_\mu''(\i x)$, and since $J_\mu$ solves \eqref{Bessel equation}, we have that
\begin{align*}
\tilde J_\mu''(x) + \frac{1}{x} \tilde J_\mu'(x) - \Bigl( 1+ \frac{\mu^2}{x^2} \Bigr) \tilde J_\mu(x) &=  - J_\mu''(\i x) + \frac \i x J_\mu'(\i x) - \Bigl( 1 + \frac{\mu^2}{x^2} \Bigr) J_\mu(\i x) \\
&= -\Bigl[ J_\mu''(\i x) + \frac{1}{\i x} J_\mu'(\i x) + \Bigl( 1 - \frac{\mu^2}{(\i x)^2}\Bigr) J_\mu(\i x)\Bigr]=0
\end{align*}
Hence, \eqref{Kmu definition} is solving \eqref{Bessel modified equation}.

Next, we want to prove that the integral representation \eqref{Kmu integral rep} also solves \eqref{Bessel modified equation}. Recall that the integral representation \eqref{Kmu integral rep} reads
\begin{align*}
K_\mu(x) = \int_0^\infty \cosh(\mu s)\e^{-x \cosh(s)} \, \ds
\end{align*}
just taking the integral on $[0, \infty)$ and collecting the emergent exponential into a $\cosh$. We need to derive this function twice. First, we have
\begin{align*}
K_\mu'(x) = - \int_0^\infty \cosh(\mu s) \cosh(s) \e^{-x \cosh(s)} \, \ds
\end{align*}
Second, we obtain
\begin{align*}
K_\mu''(x) = \int_0^\infty \cosh(\mu s) \cosh^2(s) \e^{-x\cosh(s)} \, \ds
\end{align*}
Now, in preparation for the verification, let us write $K_\mu'$ a bit differently. By integrating the $\cosh(s)$ by parts, we obtain
\begin{align*}
K_\mu'(x) &= -\cosh(\mu s) \sinh(s) \e^{-x\cosh(s)}\Big|_0^\infty \mathop + \\
&\hspace{30pt}+ \int_0^\infty \sinh(s) \bigl[\sinh(\mu s) \mu \e^{-x \cosh(s)} + \cosh(\mu s) \e^{-x \cosh(s)}(-x \sinh(s))\bigr] \, \ds
\end{align*}
Here, the first term vanishes. Now we can integrate by parts again, using the fact that $\sinh(s)\e^{-x \cosh(s)}$ has the primitive $-\frac 1x\e^{-x\cosh(s)}$. Copying the last term, we obtain
\begin{align*}
K_\mu'(x) &= -\frac \mu x\sinh(\mu s)\e^{-x\cosh(s)}\Big|_0^\infty + \frac{\mu^2}{x} \int_0^\infty \cosh(\mu s) \e^{-x\cosh(s)}\, \ds \\
&\hspace{170pt} - x\int_0^\infty \cosh(\mu s)\sinh^2(s)\e^{-x\cosh(s)}\, \ds,
\end{align*}
where, again, the first term vanishes. Inserting this into \eqref{Bessel modified equation}, we obtain
\begin{align*}
K_\mu''(x) + \frac 1x K_\mu'(x) - \Bigl( 1 + \frac{\mu^2}{x^2} \Bigr) K_\mu(x) =\hspace{-150pt}&\\
&= \int_0^\infty \cosh(\mu s) \e^{-x\cosh(s)}\bigl[ \cosh^2(s) + \frac{\mu^2}{x^2} - \sinh^2(s) - \bigl( 1 + \frac{\mu^2}{x^2} \bigr)\bigr] \, \ds =0
\end{align*}
The last equation follows from $\cosh^2 - \sinh^2 = 1$.

\subsubsection{Solutions to \texorpdfstring{(\ref{Bessel modified equation})}{(\ref{Bessel modified equation})} are unique}

Here, we just argue that the equation \eqref{Bessel modified equation} is a linear differential equation with nonconstant coefficients. Hence, solutions to the equation are unique. Uniqueness becomes manifest by the asymptotic behavior as $x \to \infty$. In our case, we require that
\begin{align}
K_\mu(x) \sim \sqrt{\frac{\pi}{2x}} \cdot \e^{-x} \qquad \qquad x\to\infty \label{Asymptotic requirement}
\end{align}
meaning that
\begin{align*}
\sqrt{\frac{2x}{\pi}} \cdot \e^{x} \cdot K_\mu(x) \xra{x\to\infty} 1.
\end{align*}

\subsubsection{Asymptotic behavior for the integral representation}

Recall the defining series of the $\cosh$, namely $\cosh(s) = \sum_{n=0}^\infty \frac{s^{2k}}{(2k)!}$. With this in mind, we have
\begin{align*}
\sqrt{\frac{2x}{\pi}} \e^x \cdot K_\mu(x) &= \sqrt{\frac{2x}{\pi}} \int_0^\infty \cosh(\mu s)\e^{-x(\cosh(s) - 1)}\, \ds\\
&= \sqrt{\frac{2x}{\pi}} \int_0^\infty \cosh(\mu s)\e^{-\frac{(\sqrt{x}s)^2}{2}} \cdot \exp\Bigl(-x \cdot \sum_{k=2}^\infty \frac{s^{2k}}{(2k)!}\Bigr) \, \ds
\end{align*}
Now, perform a change of variables $u = \sqrt{x} s$ with $\ds = \frac{1}{\sqrt{x}} \du$. Then
\begin{align*}
\sqrt{\frac{2x}{\pi}} \e^x \cdot K_\mu(x) &= \sqrt{\frac{2}{\pi}} \int_0^\infty \cosh\bigl( \frac{\mu u}{\sqrt{x}} \bigr) \e^{-\frac{u^2}{2}} \cdot  \exp\Bigl( - \sum_{k=2}^\infty \frac{u^{2k}}{(2k)! \cdot \sqrt{x}^{2k-1}}\Bigr) \, \du\\
&\xra{x\to\infty} \sqrt{\frac 2\pi} \int_0^\infty \e^{-\frac{x^2}{2}} \, \du = \sqrt{\frac 2\pi} \cdot \frac{\sqrt{2\pi}}{2} = 1
\end{align*}
Hence, the integral representation has the right asymptotic behavior.

\subsubsection{Computation of \texorpdfstring{$K_\mu$}{Kmu} with the definition \texorpdfstring{(\ref{Kmu definition})}{(\ref{Kmu definition})}}

Here, we want to compute the function $K_\mu$ in the case $\mu = \frac 32 - 1 = \frac 12$, i.e., $d =3$. Let us start by noting that for $\nu\in \Nbb$, we have
\begin{align}
\Gamma(\nicefrac 32 + \nu) = 1\cdot 3\cdot 5\cdot 7 \cdots (2\nu + 1) \cdot \frac{\sqrt{\pi}}{2^{\nu + 1}} \label{Gamma identity}
\end{align}
We prove it by induction. For $\nu = 0$, we have by a change of variables $t = x^2$, $\dt = 2x\dx$
\begin{align*}
\Gamma(\nicefrac 32) &= \int_0^\infty t^{\nicefrac 12} \e^{-t} \, \dt = -\int_0^\infty x(-2x)\e^{-x^2}\, \dx \\
&= -x \e^{-x^2} \Big|_0^\infty + \int_0^\infty \e^{-x^2} \, \dx = \frac{\sqrt{\pi}}{2}
\end{align*}
which is claimed. To prove the step $\nu \to \nu +1$, we use \eqref{functional equation Gamma} once
\begin{align*}
\Gamma(\nu + 1 + \nicefrac 32) = \Gamma(\nu + \nicefrac 32) \cdot (\nu + \nicefrac 32) = \Gamma(\nu + \nicefrac 32) \cdot  \frac{2(\nu + 1) + 1}{2},
\end{align*}
which proves the claim.

Keeping in mind equation \eqref{Hmu definition}, we need to compute $J_{\frac 12}$ and $J_{-\frac 12}$. Employing \eqref{Gamma identity}, we obtain
\begin{align*}
J_{\frac 12}(x) = \sqrt{\frac x2} \cdot \sum_{k=0}^\infty \frac{(-1)^k \cdot 2^{k+1}}{k!\cdot 3\cdot 5\cdots (2k+1)} \cdot \Bigl(\frac{x}{2}\Bigr)^{2k} = \sqrt{\frac{x}{2\pi}}\cdot  \sum_{k=0}^\infty \frac{(-1)^k \cdot 2\cdot x^{2k}}{2^k \cdot k! \cdot 3\cdot 5\cdots (2k+1)}
\end{align*}
Noting that the factor in the denominator is precisely $(2k+1)!$, we finally get
\begin{align*}
J_{\frac 12}(x) = \sqrt{\frac{2}{\pi x}} \cdot  \sum_{k=0}^\infty \frac{(-1)^k \cdot x^{2k+1}}{(2k+1)!} = \sqrt{\frac{2}{\pi x}} \cdot \sin(x)
\end{align*}
In the same manner, we treat $J_{-\frac 12}$ to get
\begin{align*}
J_{-\frac 12}(x) &= \sqrt{\frac 2x} \cdot \sum_{k=0}^\infty \frac{(-1)^k}{k!\cdot \Gamma((k-1) + \nicefrac 32)} \Bigl( \frac x2\Bigr)^{2k} = \sqrt{\frac{2}{\pi x}} \cdot \sum_{k=0}^\infty \frac{(-1)^k \cdot x^{2k}}{k! \cdot 2^k \cdot 3\cdot 5 \cdots (2k-1)}
\end{align*}
This time, the denominator equals $(2k)!$ and we obtain
\begin{align*}
J_{-\frac 12}(x) &= \sqrt{\frac{2}{\pi x}} \cdot \sum_{k=0}^\infty \frac{(-1)^k \cdot x^{2k}}{(2k)!} = \sqrt{\frac{2}{\pi x}} \cdot \cos(x)
\end{align*}

Finally, we put everything together using \eqref{Hmu definition}. We get
\begin{align*}
H_{\frac 12}^{(1)}(x) &= \sqrt{\frac{2}{\pi x}} \cdot \frac{\cos(x) - \e^{-\i \frac \pi 2} \sin (x)}{\i \sin(\nicefrac \pi 2)} = \sqrt{\frac{2}{\pi x}} \cdot \bigl[ \sin(x) - \i \cos(x)\bigr]\\
&=\frac 12 \sqrt{\frac{2}{\pi x}} \cdot \bigl[ \i \e^{-\i x} - \i \e^{\i x} - \i \e^{\i x} - \i \e^{-\i x}\bigr] = -\i \cdot  \sqrt{\frac{2}{\pi x}} \cdot \e^{\i x}.
\end{align*}
Thus, using \eqref{Kmu definition}, we end up with
\begin{align}
K_{\frac 12}(x) = \frac \pi 2 \cdot\i \e^{\frac{\pi \i}{4}} H_{\frac 12}^{(1)}(\i x) = -\frac\pi 2 \sqrt{\frac{2}{\pi\i x}}\cdot  (-1) \cdot \e^{\frac{\pi \i }{4}} \e^{-x} = \sqrt{\frac{\pi}{2x}}\cdot \e^{-x} \label{Konehalf final representation}
\end{align}
As we see from \eqref{Asymptotic requirement}, the above function has the right asymptotic behavior. Thus, it has to coincide with the integral representation \eqref{Kmu integral rep}.

%\subsubsection{Verification of the kernel property}
%
%Inspiration from MQM Sheet 8 Ex 1 \doit

\printbibliography[heading=bibliography]

\end{refsection}
