# Supplementary material for: BCS Theory in the Weak Magnetic Field Regime for Systems with Nonzero Flux and Exponential Estimates on the Adiabatic Theorem in Extended Quantum Lattice Systems
Source: arXiv:2210.04746 source file (2022-10-10)
Supplement: Supplementary file 2 [file application_to_entropy.tex]

%auto-ignore  % for ArXiv to process correctly

\section{Application to the entropy}

\begin{prop}
For $x\in [0,1]$ let $f(x) := x\ln(x) + (1 - x)\ln(1-x)$ with the convention that $\lim_{x\searrow 0 } x\ln (x) =0$. Then $f$ is strictly convex on $[0,1]$.
\end{prop}

\begin{proof}
It suffices to prove that $f'$ is strictly increasing on $(0,1)$. Computing the derivative, we have $f'(x) = \ln(x) - \ln(1 - x)$ and $f''(x) = \frac{1}{x(1-x)} >0$ for all $x\in (0,1)$.
\end{proof}

%\begin{thm}[BCS-minimizer]
%Let $\hfrak$ be a one-particle operator in $\Hcal$ and let
%\begin{align*}
%H_0 := \begin{pmatrix} \hfrak \\ &-\ov \hfrak\end{pmatrix}
%\end{align*}
%Let $\Phi(x) := x\ln(x) + (1 - x)\ln(1 - x)$ for $x\in [0,1]$ with $\lim_{x\searrow 0} x\ln(x) =0$. Define $\Gamma_0 := (1 + \e^{\beta H_0})^{-1}$ and assume that $\Gamma_0\in \Scal^1_\Phi(\Hcal \oplus \Hcal)$. Furthermore, assume that $\hfrak \Gamma_0\in \Scal^1(\Hcal)$. 
%\end{thm}
